# Supplementary material for: FFaceNeRF: Few-shot Face Editing in Neural Radiance Fields
Source: arXiv:2503.17095 source file (2025-03-21)
Supplement: Supplementary file 1 [file 99_suppl.tex]

\clearpage
\setcounter{page}{1}
\vspace{5mm}
\maketitlesupplementary

\section*{Overview}
\label{sec:Overview}
In this supplementary material, we present details of model architecture in Section~\hyperref[sec:A]{A}. Section~\hyperref[sec:B]{B} covers details of the experiments. Section~\hyperref[sec:C]{C} presents additional details and explanation of our applications. Section~\hyperref[sec:D]{D} presents an experiment on dataset scaling. Section~\hyperref[sec:E]{E} present additional experiments. Lastly, Section~\hyperref[sec:F]{F} discusses about the social impact.

% For additional results, please visit the project page~\href{https://kwanyun.github.io/lego/}{https://kwanyun.github.io/lego/}.

\section*{A. Architecture of Geometry Adapter}
\label{sec:A}
Our geometry adapter, $\Phi_{geo}$, consists of a lightweight MLP that receives the viewing direction $v_{d} \in {\Bbb R}^{3}$, the Tri-plane feature $\hat{F}'_{tri} \in {\Bbb R}^{32}$, the segmentation label of the geometry decoder $Seg \in {\Bbb R}^{15}$, and the density $\sigma \in {\Bbb R}^{1}$ in the Figure 2 of the main paper. Therefore, the input dimension is 51, and the output dimension is the number of new mask labels, which in our experiments were 17 for the Base layout and 19 for the Nose and Eyes layouts. 

To evaluate whether this simple MLP can effectively fuse different features compared to attention modules, we conducted an additional study to identify any differences. The alternative architecture replaced the first layer of our $\Phi_{geo}$ with multi-head self-attention, where the number of heads was set to 4 as shown in the Figure~\ref{fig:network}. The comparison was conducted under the same conditions as in the ablation study in Section 4.4 of the main paper. The evaluation results show that switching to the multi-head self-attention module did not have a meaningful effect (0.847 mIoU with training on 10 data, compared to 0.850 with our MLP) but did increase the training time. Therefore, we chose the MLP architecture for $\Phi_{geo}$.

\begin{figure}[h]
  \centering
  % the following command controls the width of the embedded PS file
  % (relative to the width of the current column)
  \hspace{-6mm}
  \includegraphics[width=1.05\linewidth]{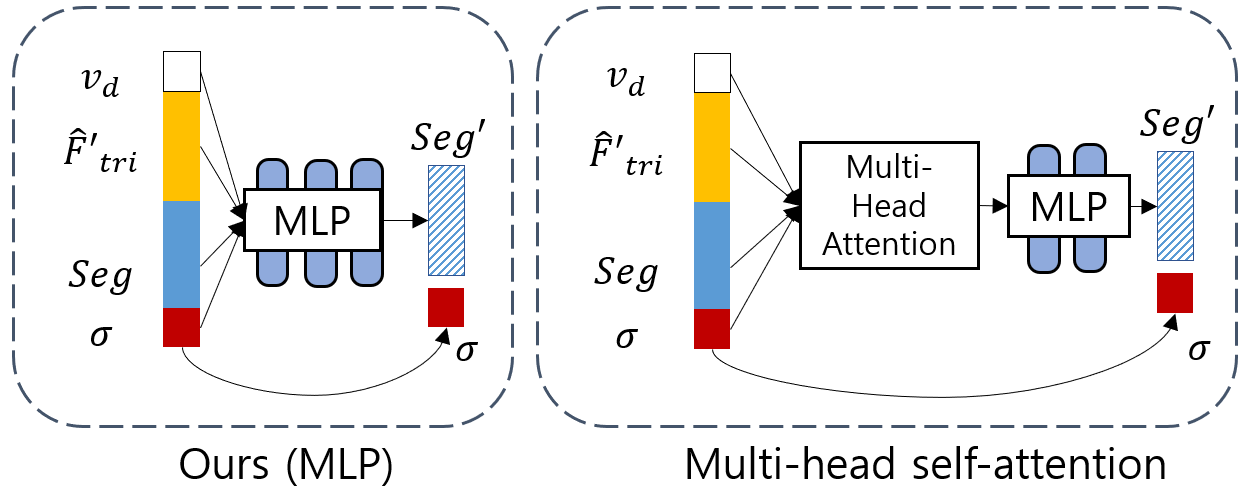}
  \vspace{1mm}
  \caption{Visualization of our MLP network and multi-head self-attention network which are used as the geometry adapter.}\label{fig:network}
\end{figure}

\section*{B. Additional Details of Experiments}
\label{sec:B}
\subsection*{B.1 Tri-plane Mixing}

We conducted tri-plane mixing experiments in Section 4.3 of the main paper and found a balance between the tri-plane mixing ratio and augmentation effectiveness. We considered two variables, mIoU and L1, each representing the retention of semantic information and the variance of information, respectively. Using these variables, we identified the top layers for each variable, as shown in Table~\ref{tab:top6_layers}. For instance, referring to Table~\ref{tab:top6_layers}, when N=2 layers were mixed for the top mIoUs, we combined layers 13 and 14. When N=5 layers were mixed for mIoU, we combined layers 10 through 14 (13, 14, 11, 12, and 10). Similarly, when N=5 layers were mixed for the top L1, we combined layers 1 through 5.

\begin{table}[h]
\centering
\setlength{\tabcolsep}{5mm}
\caption{List of the top 7 layers in mIoU and L1, respectively} %{-10pt}
\small
\begin{tabular}{|c|c|}
\noalign{\smallskip}\noalign{\smallskip}\hline
mIoU & L1  \\
\hline
13 & 5 \\ 
14 & 1 \\
11 & 2 \\
12 & 4 \\
10 & 3 \\
9 & 6 \\
8   & 7   \\
% 2   & 8   \\
% 6   & 9   \\
% 1   & 10   \\
% 4   & 12   \\
% 3   & 14   \\
% 7   & 11   \\
% 5   & 13   \\
\hline
\end{tabular}
\label{tab:top6_layers}
\end{table}

\subsection*{B.2 Baseline Comparisons}
We compared our method with two masked based face editing methods: NeRFFaceEditing~\cite{jiang2022nerffaceediting} and IDE-3D~\cite{sun2022ide}.
For NeRFFaceEditing, we fine-tuned the model by training only the geometry decoder while keeping the other components fixed.
This approach was necessary because training the entire model with only 10 data samples, as in our method, led to overfitting.
Similarly, for IDE-3D, we trained only the semantic decoder.
Note that the geometry decoder in NeRFFaceEditing and the semantic decoder in IDE-3D serve similar roles, though they are named differently in their respective papers. In addition to the comparison results included in the main paper, we present additional editing results produced by our FFaceNeRF and two baselines, in the upper part of Figure~\ref{fig:x_comp}.

\begin{figure*}[t]
  \centering
    \vspace{-3mm}
  \includegraphics[width=0.95\linewidth]{figures/x_comparison_final.png}
  \caption{Additional comparison results between our method, two baseline methods, and two additional methods. NeRFFaceEditing showed degraded quality with texture shifts and incomplete editing, particularly on elements like clothing. IDE-3D failed to reconstruct identity, FaceEdit3D failed to edit undefined regions, and InstructPix2NeRF exhibited limited control. In contrast, our method faithfully edited the source image in accordance with the target mask.}
  \label{fig:x_comp}
\vspace{-1mm}
\end{figure*}

\subsection*{B.3 Comparisons with Other Editing Methods} 
Mask-based editing offers distinct advantages over other face editing methods, particularly in its ability to achieve detailed and precise modifications. Unlike point-based, text-based, or sketch-based approaches, mask-based methods enable fine-grained control by explicitly defining regions for edits. To demonstrate this, we conducted additional experiments comparing our approach with text-based and point-based editing methods~\cite{li2024instructpix,cheng20243d}.

FaceEdit3D~\cite{cheng20243d} is a point-based editing method that warps the tri-plane to determine the editing direction in the latent space. When using this method, use of excessive control points may lead to distortions. To mitigate this, FaceEdit3D allows to use predefined landmarks only, making edits outside these points impossible. InstructPix2NeRF~\cite{li2024instructpix}, a state-of-the-art text-based 3D face editing method, can perform edits using natural language prompts. Due to the nature of text prompts, controlling the range or specificity of edits is challenging with this method. 
SketchFaceNeRF~\cite{gao2023sketchfacenerf} is a sketch based 3D face editing method, that can either generate face from sketch and edit randomly generated face using sketch. However this model does not provide method to edit face from arbitrary face, therefore we randomly generated a face and edit the images to visualize.

\begin{figure}[t]
  \centering
  % the following command controls the width of the embedded PS file
  % (relative to the width of the current column)
  \includegraphics[width=0.8\linewidth]{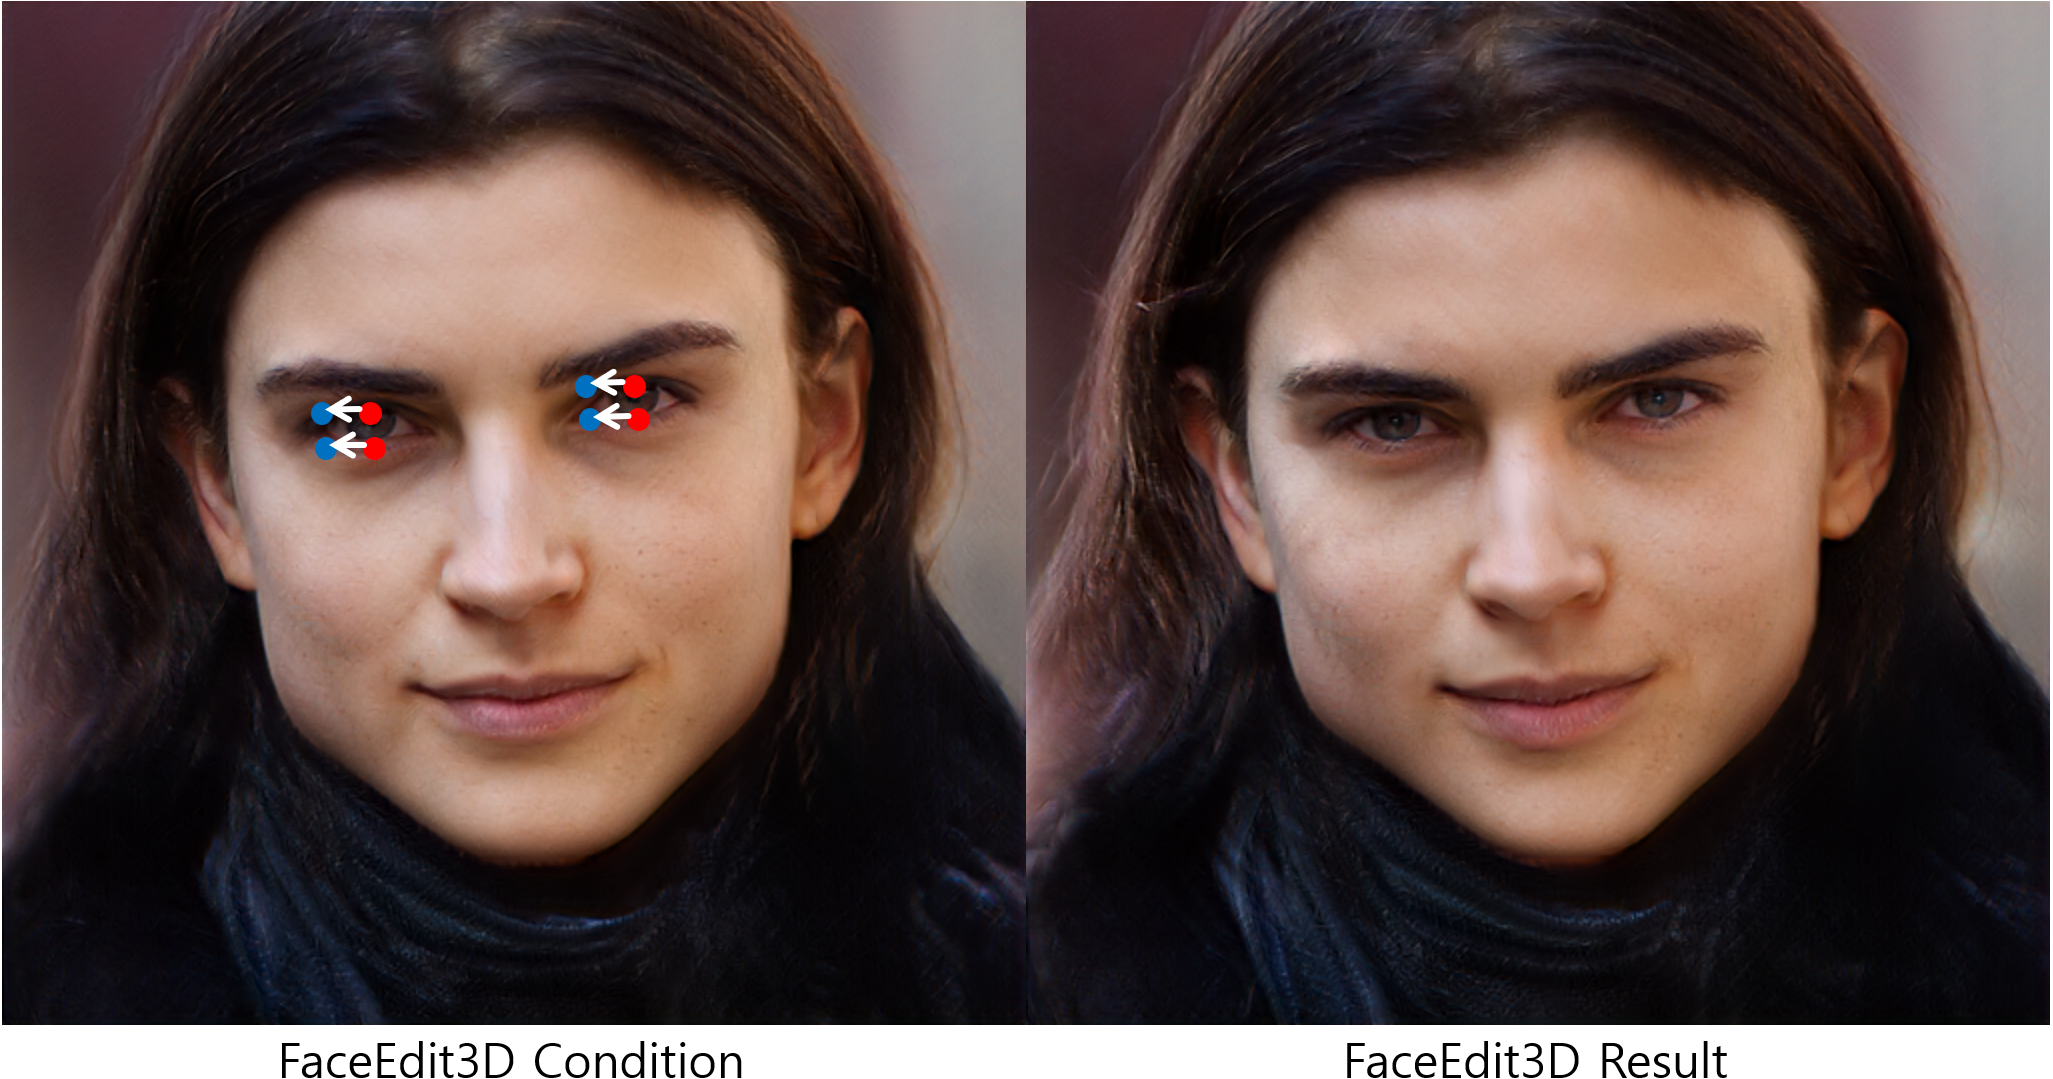}
  \caption{Gaze direction editing results of FaceEdit3D.}
  \label{fig:x_faceedit}
  \vspace{-3mm}
\end{figure}

\begin{figure}[h]
  \centering
  \includegraphics[width=\linewidth]{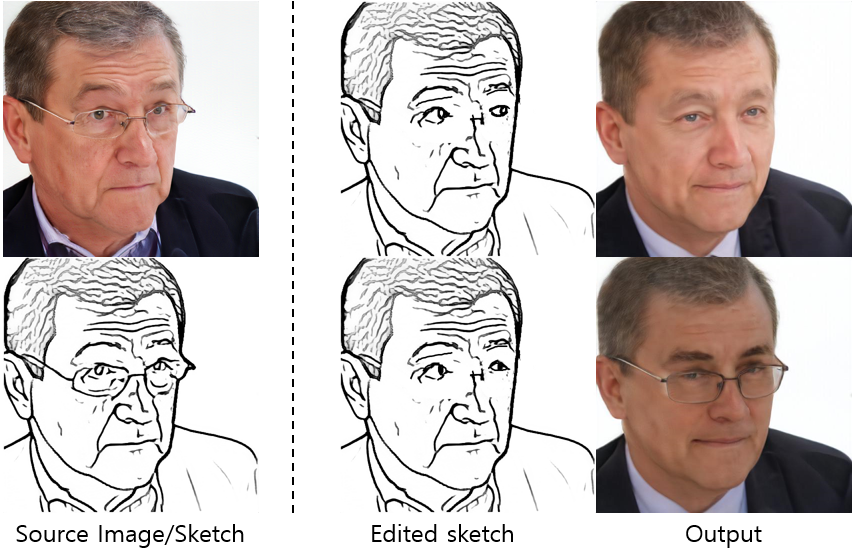}
   \vspace{-2mm}
   \caption{Gaze direction editing results of SketchFaceNeRF. Left shows source image and corresponding sketch, while right shows edited sketch and corresponding output face.}
   \label{fig:sketchface}
   \vspace{-1mm}
\end{figure}

Visual comparison results are shown in the lower part of Figure~\ref{fig:x_comp}. While FaceEdit3D~\cite{cheng20243d} successfully edited the mouth, it failed to edit clothing because there were no control points on the neck or clothing. Similarly, gaze direction could not be edited, as shown in Figure~\ref{fig:x_faceedit}. On the other hand, InstructPix2NeRF~\cite{li2024instructpix} was able to generate both samples, but the generated images did not consistently follow the given prompts. Additionally, similar contexts with different prompts often produced inconsistent outputs. Visual results of SketchFaceNeRF are presented in Figure~\ref{fig:sketchface}. Starting from the randomly generated image (top left), we edited the image using two sketches (middle) to modify the eye gaze while removing the glasses. Although the results on the top right successfully removed the glasses, both trials failed to modify the eye gaze because the pupil is a very small region in the overall sketch, limiting to change the eye gaze using the sketch based model.

\subsection*{B.4 Statistical Analysis} 
We conducted statistical analysis on user study to verify significance compared to baselines. We conducted a Chi-Square Goodness-of-Fit test followed by a two-proportion z-test as a post-hoc analysis. Null hypotheses for all evaluation metrics were rejected in Chi-Square Goodness-of-Fit test (all p$<$0.001). The post-hoc analysis was performed only to compare our method with the competitors’. As shown in Figure~\ref{fig:statistic}, all differences in choices were statistically significant (p$<$0.001), denoted by ***.

\begin{figure}[h]
  \centering
  \includegraphics[width=\linewidth]{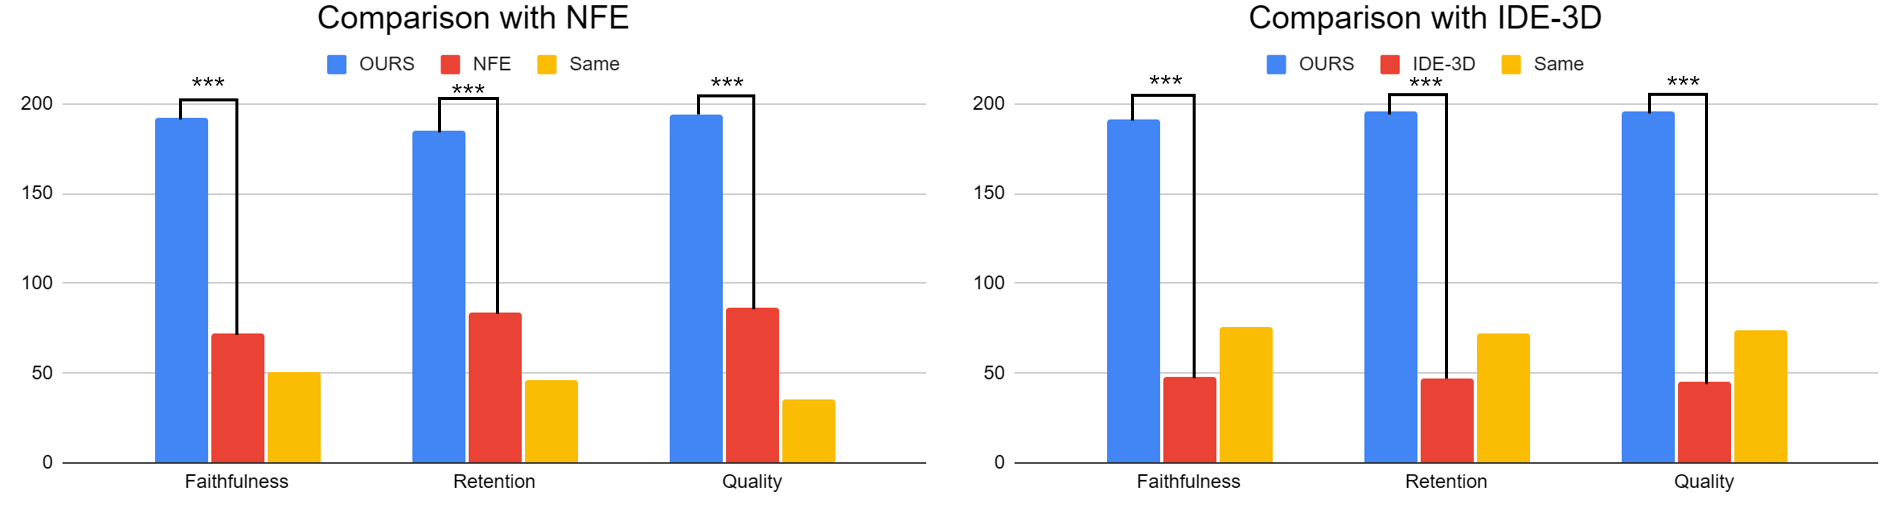}
   \vspace{-2mm}
   \caption{User study analysis results.}
   \label{fig:statistic}
   \vspace{-1mm}
\end{figure}

\begin{figure}[t]
  \centering
  % the following command controls the width of the embedded PS file
  % (relative to the width of the current column)
  \includegraphics[width=\linewidth]{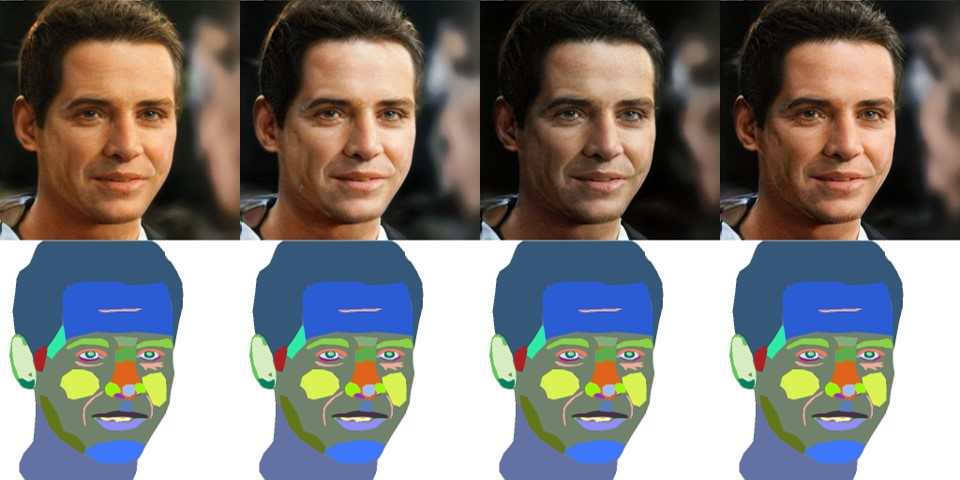}
  \caption{Visualization of augmentation results, which show color changes but preservation of the semantics of the source image.}\label{fig:x_aug}
\end{figure}

\section*{C. Additional Details of Applications}\label{sec:C}
\subsection*{C.1 Partial Style Transfer}
As stated in the main paper, our method can be utilized for a partial style transfer application. We extracted the mean and variance of the tri-plane from style images, and denormalized the source tri-plane for the full style transfer. Here, $I$ indicates the source image and $I_{stylized}$ indicates the fully stylized image. By passing the normalized source tri-plane to $\Phi_{geo}$ followed by $\Psi_{geo}$, we can obtain the resulting mask. A certain mask $M_{part}$ (such as eyes, iris, hair, or mixture of them) can be directly applied to $I_{stylized}$ for partial stylization. This can be written as follows:
\begin{align}
\small
\nonumber
M_{add} &= \sum^{parts}  M_{parts}, \ M_{apply} = \text{smooth}_w(M_{add}) \\ 
I_{partial} &= \sum^{parts} M_{apply}*I_{stylized} + (1-M_{apply})*I
\end{align}
\normalsize
where $M_{add}$ is simply added masks across parts, $\text{smooth}_w$ is linear smoothing applied to the edge of the mask with the width of $w$, where it was set to 11 in our application. Additional results are presented in Figure~\ref{fig:x_app}.

\subsection*{C.2 FFaceGAN}
To demonstrate the effectiveness of our geometry adapter, feature injection, and LMTA, we conducted experiments by incorporating an adapter module and LMTA to the DatasetGAN~\cite{zhang2021datasetgan}, resulting FFaceGAN. For the adapter, we used the same 15 BiseNet~\cite{yu2018bisenet} labels as our FFaceNeRF for the pretraining of DatasetGAN. After training DatasetGAN with the pretrained network, we froze all the parameters and added a trainable adapter, which receives the output of the original segmentation labels and the StyleGAN features as input. Because DatasetGAN uses a StyleGAN backbone instead of EG3D, there are no view direction or density values. Therefore, we only used the output label of the original segmentation network and the StyleGAN features. We trained our adapter in the same way as the original DatasetGAN.

For the augmentation strategy LMTA, we randomly sampled latent $w'^+$ and mixed with $w^+$ from training set at the last five layers, as performed for the original FFaceNeRF. To assess whether mixing the last five layers still provides correct augmentation, we added visualizations in Figure~\ref{fig:x_aug}. The results indicate that the mixing strategy of FFaceNeRF can still be applied to DatasetGAN, changing the color without altering the semantics. The results of FFaceGAN are shown in Figure~\ref{fig:x_app2}, demonstrating that our adapter and augmentation strategy can effectively enhance performance, even with different architectures.

\begin{figure}[t]
  \centering
  \includegraphics[width=\linewidth]{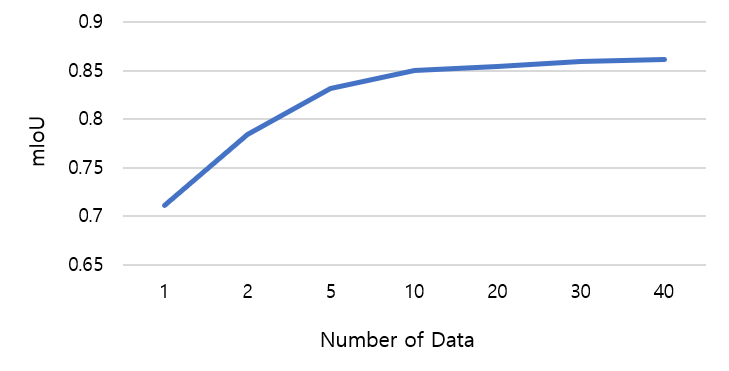}
  \vspace{-5mm}
  \caption{Number of data used for training and resulting mIoU values. The mIoU value increases as the number of training data used becomes larger. }
  \label{fig:fig_scaling}
\end{figure}

\section*{D. Dataset Scaling}\label{sec:D}\vspace{-1mm}
We conducted an additional study to investigate how the number of data used to train our model affects the performance. We varied the number of training data $n \in [1,2, 5, 10, 20, 30, 40]$ from the Base dataset. %We additionally plot the NeRFFaceEditing, calculated in Sec.~\ref{sec:baseline} for visualization.
As shown in Figure~\ref{fig:fig_scaling}, the mIoU value increased as the number of training data increased up to 40. Even with a small dataset of 5 or 10 samples, the performance was already acceptable for use, and it improved incrementally as the number of training samples increased beyond 20.

\section*{E. Additioanl experiments}\label{sec:E}
\subsection*{E.1 Additional Data}
To further validate our model, we built a new layout called Mouth by adding teeth, jaw, and chin components. The current FFaceNeRF model was pretrained on 15 layouts and supports four different layouts for training and testing: Base, Eyes, Nose, and Mouth. While Base has 17 layouts, Eyes and Nose have 19 layouts, and Mouth has 20 layouts. Results produced using our Mouth layout for accessory adoption and teeth exposure are shown in Figure~\ref{fig:mouth}.

\begin{figure}[h]
  \centering
      \includegraphics[width=\linewidth]{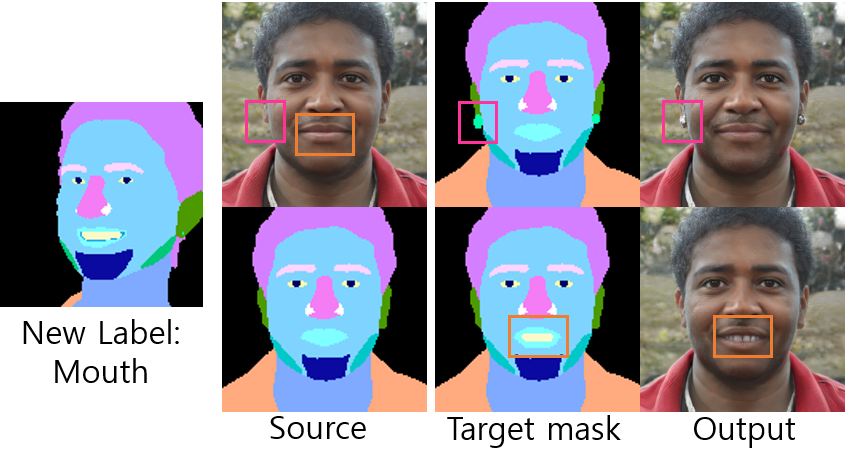}
      \vspace{-1mm}
      \caption{Editing results trained on new label "Mouth". Top: Accessories adoption, Bottom: Teeth.}
      \label{fig:mouth}
      \vspace{2mm}
\end{figure}

Furthermore, our original Base dataset consisted of a training set of 40 examples and a test set of 22 examples. We built an expanded dataset by adding an additional 20 test examples to ensure robust testing. In addition to the original dataset, we made this additional dataset publicly available.
%We conducted additional experiment of FFaceNeRF on this expanded dataset in Table~\ref{}. In addition to original dataset, we made this additional dataset publically available.}

\begin{table}[t]
\centering

\setlength{\tabcolsep}{2mm}
\caption{Quantitative results of ablation study on mask generation with a different number of training data. The highest scores are denoted in bold.}\vspace{-3mm}\small
\begin{tabular}{|l|c|c|c|c|c|c|}
\noalign{\smallskip}\noalign{\smallskip}\hline
Number of Data & 1 & 5 & 10 & 20 & 30 \\
\hline
Ours                  & 0.711 & \textbf{0.832} & \textbf{0.850} & \textbf{0.855} & \textbf{0.860} \\ 
w/o injection & \textbf{0.741} & 0.806 & 0.835 & 0.844 & 0.847 \\ 
\hline
\end{tabular}
\vspace{-4mm}
\label{Tab:ablation}
\end{table}

\begin{figure*}[t]
  \centering
  \includegraphics[width=\linewidth]{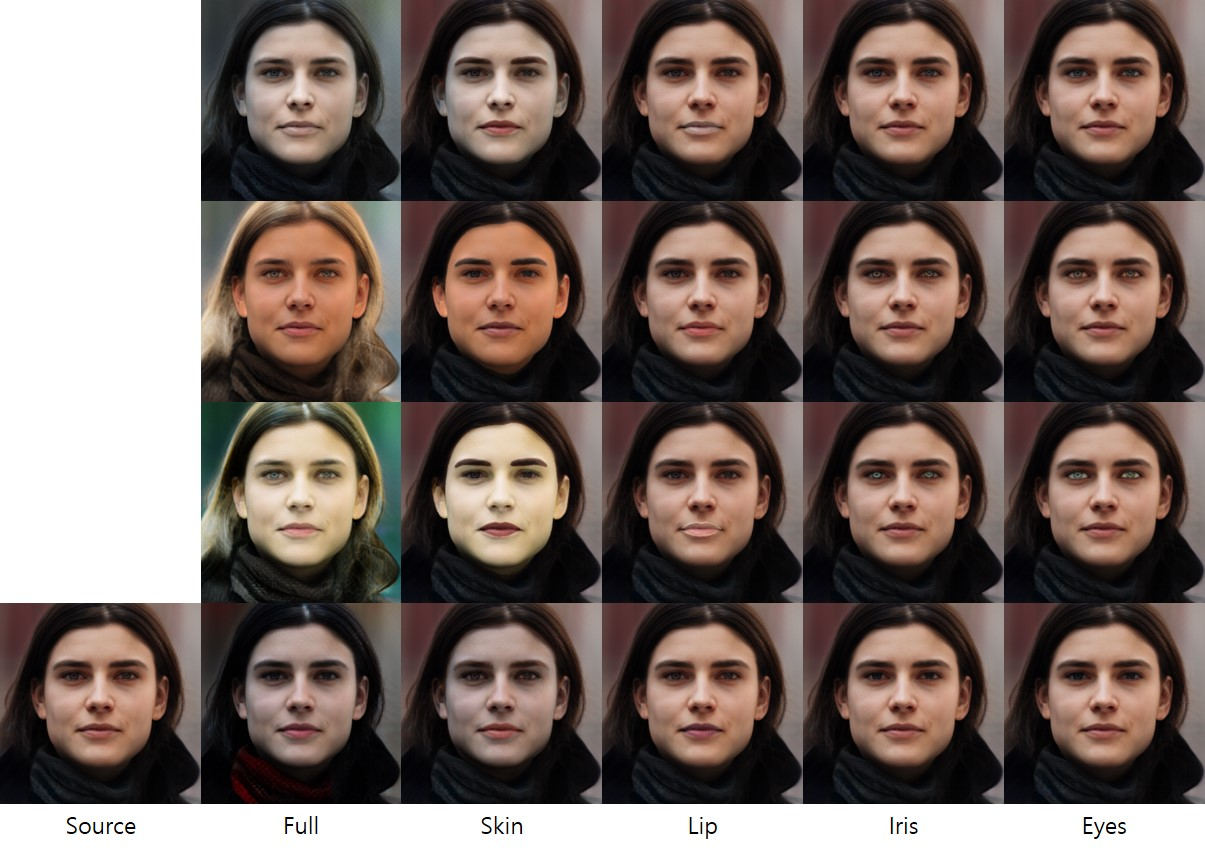}
  \vspace{-5mm}
  \caption{Visualization of partial style transfer.}\label{fig:x_app}
\end{figure*}

\begin{figure*}[h]
  \centering
  % the following command controls the width of the embedded PS file
  % (relative to the width of the current column)
  \includegraphics[width=\linewidth]{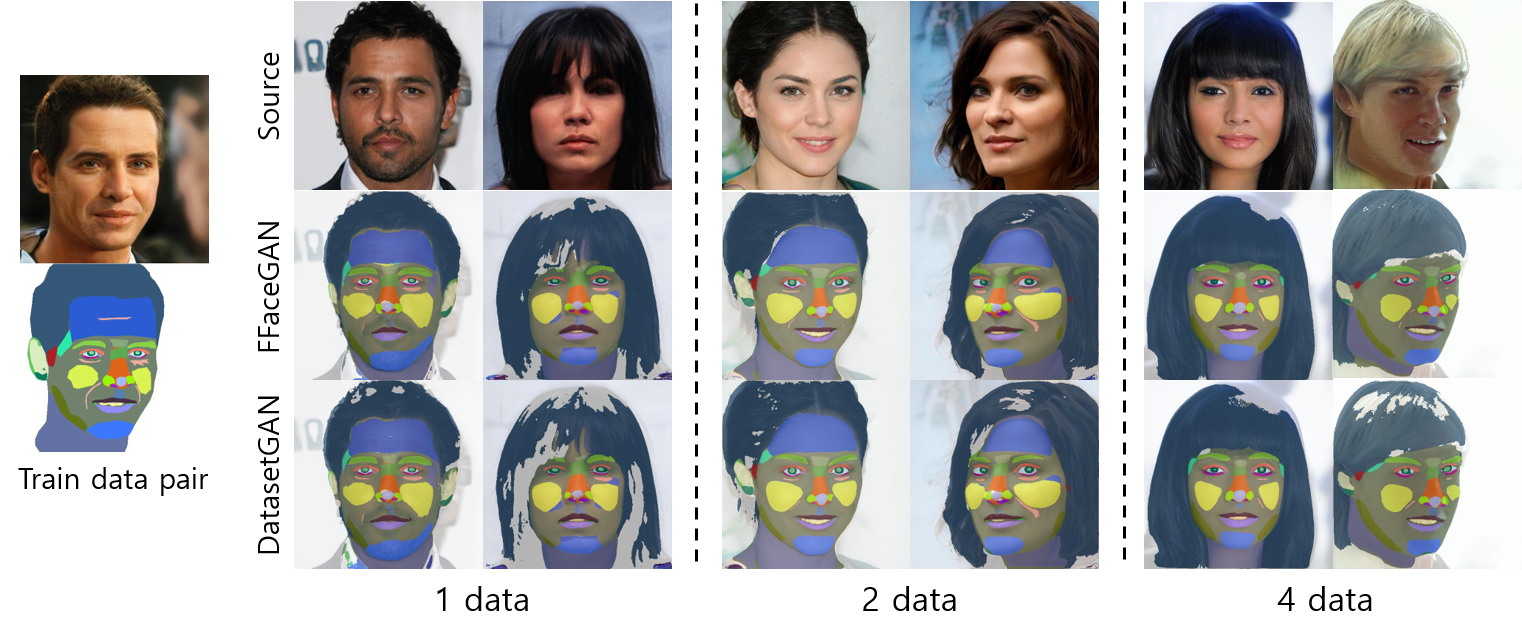}
  \vspace{-5mm}
  \caption{Comparison of results produced by our FFaceGAN and the original DatasetGAN. This indicates effectiveness of our adapter and augmentation strategy.}\label{fig:x_app2}
\end{figure*}

\section*{F. Social Impact}\label{sec:F}
The introduction of FFaceNeRF presents a substantial positive impact on fields such as personalized medical imaging, virtual reality, and the creative arts by allowing precise and customizable 3D face editing with minimal training data. However, the potential for misuse, such as in the creation of identity manipulation, underscores the need for careful and responsible usage. While the overall societal impact of FFaceNeRF is positive, we will include appropriate ethical guidelines and safeguards to our released code. This will ensure that the technology is used to drive innovation and enhance user experiences while minimizing potential risks and protecting individuals' privacy and security.

\clearpage
\begin{figure*}[!t]
  \centering
  \vspace{3mm}
  \hspace{-7mm}
  \includegraphics[width=1.05\linewidth]{figures/X_ours.png}

  \caption{Additional results of FFaceNeRF in multi-view.}\label{fig:x_ours}
  
\end{figure*}
\clearpage
